# Supplementary material for: From Prompts to Pavement Through Time: Temporal Grounding in Agentic Scene-to-Plan Reasoning
Source: arXiv:2605.19824 source file (2026-05-19)
Supplement: Supplementary file 1 [file 7_appendix.tex]

\appendices
\section{Proof of the First Zonklar Equation}
Appendix one text goes here.

% you can choose not to have a title for an appendix
% if you want by leaving the argument blank
\section{}
Appendix two text goes here.
